# Supplementary material for: Xapagy: a cognitive architecture for narrative reasoning
Source: arXiv:1105.3486 source file (2011-05-17)
Supplement: Supplementary file 1 [file AppendixRoadsNotTaken.tex]

There is no question of the validity of these effects at the outside level. The questions is whether the effects are present in an intrinsic way at the level of instances and verb instances, or whether they are an emergent property of the architecture. Note than in Xapagy a recalled story creates a new, similar story in addition to the already recorded one. The collection of these stories make for a stronger shadow. 

\medskip

To avoid misunderstandings, we need to state here that only the explicit recall of the story creates a new story, shadowing does not. 

Shadow is not part of conscious thought. We cannot introspect on the shadow, but we can introspect on all the elements of the focus - they can form parts of new verb instances.

% *********************************************************
%
%   Priming
%
% *********************************************************

\subsubsection{Priming}

Priming makes certain memories more likely to recall in certain situations. Without any further intervention, the Xapagy system exhibits priming by the impact of story chains already in the shadow. 

The question here is whether there is any other mechanism needed beyond the ones provided by the shadowing mechanism.
